# Supplementary material for: MonoGSDF: Exploring Monocular Geometric Cues for Gaussian Splatting-Guided Implicit Surface Reconstruction
Source: arXiv:2411.16898 source file (2025-11-20)
Supplement: Supplementary file 1 [file supp.tex]

\begin{table}[t]
\centering

\resizebox{.38\textwidth}{!}{
\begin{tabular}{@{}lccc}
    \hline
          Method & w/ MipNeRF NF & w/ 3DGSR SDF2O & \textbf{Ours} \\
    \hline
         F-score & 0.52 & 0.24 & \textbf{0.56} \\
    \hline
\end{tabular}
}
\caption{
\textbf{Ablation Study on Normalization and SDF to Opacity.} We show the F-score of reconstructed mesh on Barn.
}
\label{tab:supp}
\end{table}
